# Supplementary material for: NeuralFastLAS: Fast Logic-Based Learning from Raw Data
Source: arXiv:2310.05145 source file (2023-10-08)
Supplement: Supplementary file 1 [file appendix.tex]

\appendix

\section{Details of the Solving Stage}

\subsection{Constructing the Program}
\label{appendix:psolve}

$P_\text{solve}$ consists of the following elements:

\begin{enumerate}
  \item \label{item:opt1} For each hypothesis $h \in \smopt$,
  we add to $P_\text{solve}$ the choice rule and weak constraint:
\begin{code}
0 { in_h(h(*$_\text{id}$*)) } 1.
:~ in_h(h(*$_\text{id}$*)).[(*$ \abs{E} \abs{H } $*)@1, in_h(h(*$_\text{id}$*))]
\end{code}
  \item For each example $e \in E$, we have the constraint 
\begin{code}
    :- not covered(e(*$_\text{id}$*)).
\end{code}
  Furthermore, we say that an example is covered 
  if at least one of its possibility groups is 
  covered and a possibility group is covered if at least
  one of its possibilities is covered.

  Each possibility group corresponds to a 
  latent labelling $z \in \Z$. In ASP, we
  will identify $z$ by  $\texttt{z}_\text{id}$.
  For each possibility group $pp_z$, we perform the following:
  Add the rule
    \begin{code}
covered(e(*$_\text{id}$*)) 
(*\null*)    :- pgroup_covered(e(*$_\text{id}$*),z(*$_\text{id}$*)).
    \end{code}
  Then, for each possibility $\texttt{p} \in pp_z$, we add the rule
    \begin{code}
pgroup_covered(e(*$_\text{id}$*),z(*$_\text{id}$*)) 
(*\null*)    :- not poss_not_covered(p(*$_\texttt{id}$*)).
    \end{code}
  Add the atom 
    \begin{code}
    poss_group_penalty(e(*$_\text{id}$*),z(*$_\text{id}$*),(*$P_\theta (z | x)$*)).
    \end{code}
  For each $\texttt{p} \in pp_z$, to define \texttt{poss\_not\_covered}, we use the same 
    logic as in \autoref{subsec:fl_solve}: Define for convenience
    \begin{align*}
      O^+(a, \texttt{p}) &= \{ h : h \in \smopt,\ \exists r \in C^+(T, a, \texttt{p}). h \leq r \}
      \\ O^-(a, \texttt{p}) &= \{ h : h \in \smopt,\ \exists r \in C^-(T, a, \texttt{p}). h \leq r \}
    \end{align*}
  Then we create the rules 
    \begin{code}
      poss_not_covered(p(*$_\texttt{id}$*)) 
(*\null*)    :- (*$\bigwedge_{\texttt{h} \in O^+(\texttt{a}, \texttt{p})}$*) not in_h(h(*$_\texttt{id}$*)).
    \end{code}
    and for each $\texttt{a} \in \texttt{p}_\text{pi}^\text{exc}$ and $\texttt{h} \in O^-(\texttt{a}, \texttt{p})$, we add the rule 
    \begin{code}
      poss_not_covered(p(*$_\texttt{id}$*)) :- in_h(h(*$_\texttt{id}$*)).
    \end{code}
  \end{enumerate}
  Finally, we add the rule 
  \begin{code}
  min_ex_penalty(Ex, Pen) 
  (*\null*)  :- example(Ex), 
  (*\null*)     Pen=#min{P : pgrp_cov(Ex, Z), 
  (*\null*)                  pgrp_pen(Ex, Z, P)}.
  \end{code}
  and the weak constraint 
  \begin{code}
  :~ min_ex_penalty(Ex, P).[P@1, Ex].
  \end{code}
  With this weak constraint combined with the 
  weak constraint defined in 
  \hyperref[item:opt1]{Step 1}, Clingo will 
  attempt to minimize over the sum of the 
  hypothesis size penalty and the minimum 
  example penalties which is consistent with 
  \autoref{eq:nfl_opt}.

\section{Semantic Loss in Neural FastLAS}

To generate the answer sets to compute the semantic 
loss with respect to $y$, let $P$ be the program defined 
in \autoref{def:asp_semantic}. We add to $P$ the following 
components to create $P_y$:
\begin{enumerate}
  \item 
  We use the constraint 
  \begin{code}
  :- not (*$y$*).
  \end{code}
  to restrict the answer sets only to those that prove $y$.
  \item For each rule $r_i \in \smopt$, we add the following 
  rule to $P$:
  \begin{code}
  (*$\head(r_i)$*) :- use((*$i$*)), (*$\body(r_i)$*).
  \end{code}
  \item Since NeuralFastLAS tasks are non-recursive and 
  do not have chaining of learnt rules (i.e. \texttt{p :- q. q :- r.}
  is a chain of learnt rules), then for a
  given label, we only need to use one rule to derive the 
  label from the background knowledge.
  Therefore, we have the 
  choice rule 
  \begin{code}
    1 { use(0..M) } 1.
  \end{code}
  where $\texttt{M} = \abs{\smopt}$, so each of the generated 
  answer sets corresponds directly to one of the rules in 
  $\smopt$. 
\end{enumerate}

\section{Semantic Loss}

In this section, we explain the mechanism we use 
to compute the semantic loss with $p_\theta(z | x)$
and $p(r | \theta_R )$. Suppose we have an 
example 
$e = \langle e_\text{id}, 
\langle \epi^\text{inc} , \epi^\text{exc} \rangle, 
e_\text{ctx}, e_\text{raw} \rangle$ and neural 
network parameters $\theta$ and $\theta_R$, we 
define the atoms $X_i$ for the semantic loss by:
\begin{equation}
  X_i = \begin{cases}
    \texttt{use(}i\texttt{)} & \text{for $i < \abs{\smopt}$} \\
    \texttt{nn(}j\texttt{, }k\texttt{)} & \text{otherwise, where $i = \abs{\smopt} + j n + k$}
  \end{cases}
\end{equation}
where $n$ is the number of latent concepts for each 
raw data input. In essence, the first $\abs{\smopt}$ 
elements mapped to by $X_i$ represent possible 
choices for rules, and the rest of the elements 
represent the enumeration over the possible latent 
concept labels. Note that in the second case, $j$ 
starts from $0$ and $k$ indexes the possible 
latent concept values.

\section{Experiment Configurations}
\label{app:experiments}
